# Supplementary material for: A smile is all you need: Predicting limiting activity coefficients from SMILES with natural language processing
Source: arXiv:2206.07048 ancillary file (2022-06-15)
Supplement: Supplementary file 1 [file SI_a_smile_is_all_you_need.pdf]

# Supporting Information:
# A SMILE is all you need:
# Predicting limiting activity coefficients from SMILES with natural language processing

## S1: Vocab

Table S1 contains the vocab used to train SPT. The X in the table signifies if an embedding is contained in the training data and thus is trained in the provided model. Predicting ln γ for molecules with untrained embeddings leads to unreliable results.

*Table S1: Vocab used for the model. The Trained column indicates whether the character is contained in the training datasets X.*

| Index | Char | Trained | Index | Char | Trained | Index | Char | Trained |
|---|---|---|---|---|---|---|---|---|
| 0 | <pad> | X | 21 | 4 | | 42 | 8 | |
| 1 | <sos> | X | 22 | S | X | 43 | L | |
| 2 | <mos> | X | 23 | l | X | 44 | A | |
| 3 | <eos> | X | 24 | / | | 45 | Z | |
| 4 | c | X | 25 | s | X | 46 | g | |
| 5 | C | X | 26 | O | X | 47 | M | |
| 6 | ( | X | 27 | + | X | 48 | T | |
| 7 | ) | X | 28 | 5 | | 49 | T | |
| 8 | 1 | X | 29 | # | X | 50 | 9 | |
| 9 | O | X | 30 | . | | 51 | p | |
| 10 | 2 | X | 31 | B | X | 52 | % | |
| 11 | = | X | 32 | r | X | 53 | 0 | |
| 12 | N | X | 33 | \ | | 54 | V | |
| 13 | n | X | 34 | P | X | 55 | b | |
| 14 | 3 | | 35 | 6 | | 56 | u | |
| 15 | [ | X | 36 | I | X | 57 | R | |
| 16 | ] | X | 37 | a | | 58 | X | |
| 17 | @ | | 38 | i | | 59 | <H2O> | X |
| 18 | H | | 39 | 7 | | | | |
| 19 | F | X | 40 | e | | | | |
| 20 | - | X | 41 | K | | | | |

## S2: Dataset Changes

In the following, all changes conducted to the original Brower dataset are described. The updated data is available in Brouwer_dataset_adapted.xlsx.

Alessi (1984) - Chemical Engineering Communications (1984), 27(1-2), 59-67

- Date in excel was converted to a date format ➔ Corrected

Thomas (1982) - J. Chem. Eng. Dab 1982, 27, 399-405

- Line slipped ➔ Corrected

Sherman (1996) - Ind. Eng. Chem. Res. 1996, 35, 1044-1058

- Multiple exponents are missing in original data ➔ All data removed

Panneerselvam (2018) - J. Chem. Eng. Data 2018, 63, 4552–4559

- CAS Number corrected

Dohnal (2006) - J. Phys. Chem. Ref. Data, Vol. 35, No. 4, 2006

- The data for methanol in the Brouwer table did not match Dohnal et. ➔ Corrected to the values of Dohnal et al.

Schiller (1992) - J. Chem. Eng. Data 1992,37,503-508

- The paper considers commercial solvents (Genosorb 300 and Genosorb 1843) instead of pure components ➔ All data removed

## S3: Training data distribution

Figure S1 shows the temperature and ln γ distribution of the Brouwer and COSMO dataset. The distribution of the COSMO dataset covers a larger range of ln γ than the Brouwer dataset. Furthermore, the distribution of ln γ is more symmetrical for the synthetic data. For the distribution, most experimental data points are available for 298.15 K. The COSMO data has the most data points at 298.15 k due to our sampling procedure.

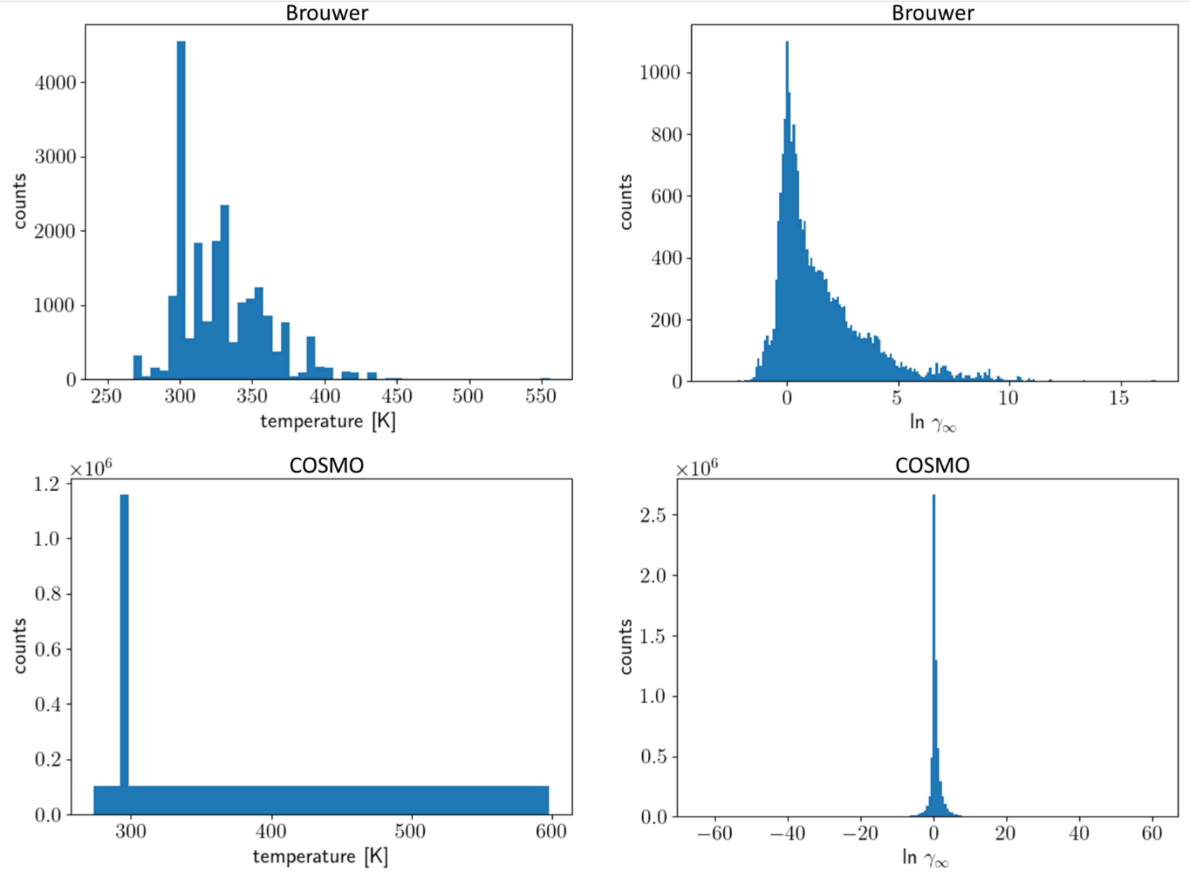


*Figure S1: Temperature and ln γ distribution of the Brouwer and COSMO datasets*

## S4: Training and model hyperparameters

Table S2-S3 shows the hyperparameters used for SPT. Hyperparameters were chosen in a manual scan to minimize the MSE of $Val_{ext}$ during pretraining. Further increasing embedding size or the number of layers slowed down the training time while not reducing MSE. Increasing embedding size past 2048 leads to divergence of the model. However, these effects might be countered by a lower learning rate. A learning rate of 1e-3 was found to perform well.

*Table S2: Hyperparameters of the model architecture*

| **Model parameters** | |
|---|---|
| Embedding size | 512 |
| Number of heads | 16 |
| Number of attention layers | 2 |
| Dropout | 0 |

*Table S3: Hyperparameters of the pretraining. For fine-tuning, learning rate was decreased by a factor of 10 to 1e-4 and batch size was decreased to 256*

| **Training parameters** | |
|---|---|
| Loss Function | MSE |
| Batch size | 1024 |
| Learning rate | 1e-3 |
| Epochs | 50 |
| Warmup epochs | 5 |
| Warmup lr increase | 100 |
| Weight decay | 0 |

## S5: Progression of training loss

Figure S2 shows the progression of the loss during pretraining.

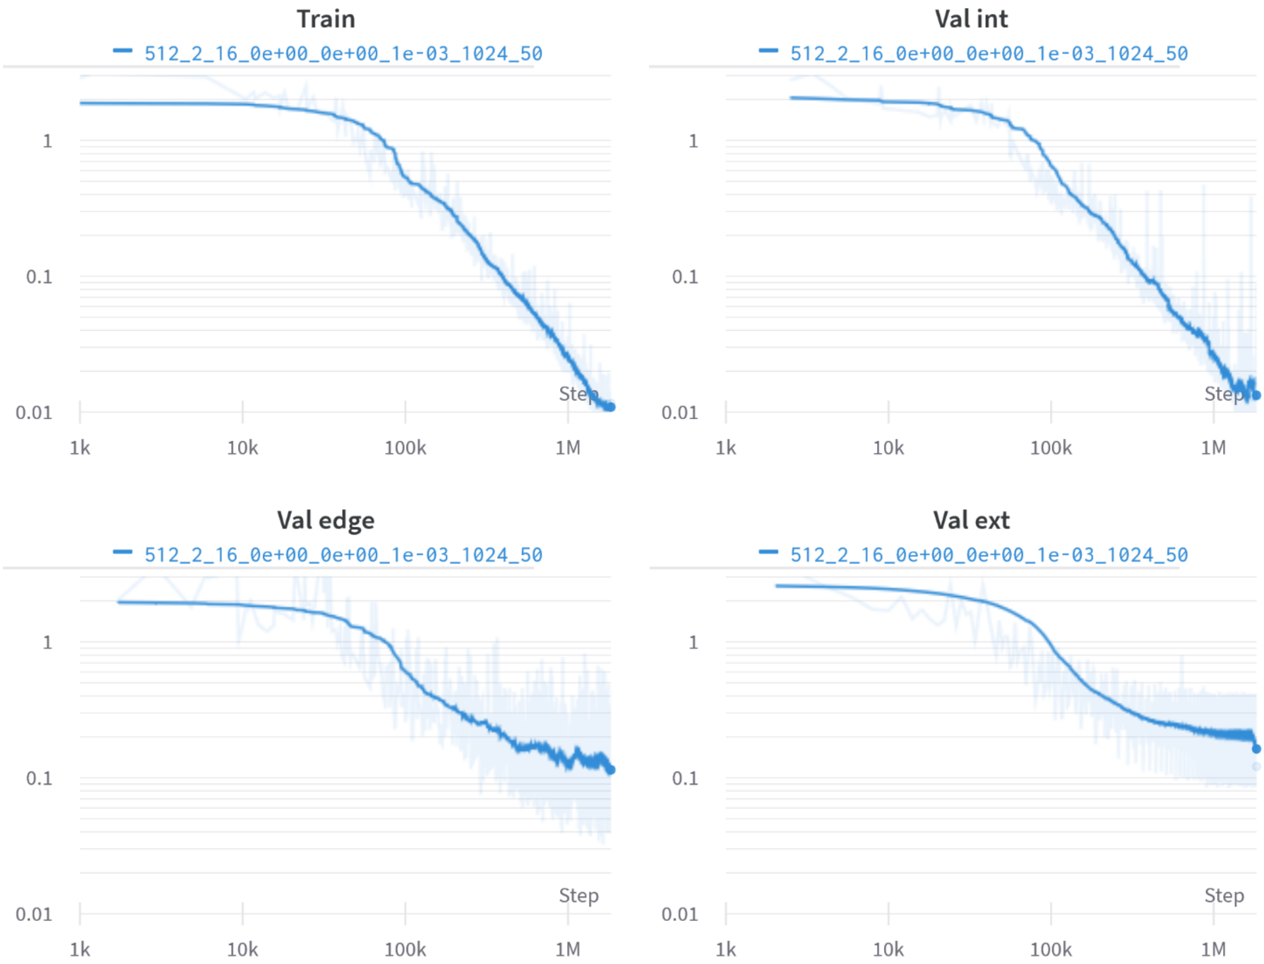


*Figure S2: Development of the loss during the pretraining. X-axis shows the training steps. $Val_{ext}$ reaches saturation during training and shows no further improvement. Continuing the training would lead to overfitting and an increase in $Val_{ext}$. $Val_{edge}$ still shows slight improvement, while $Val_{int}$ still shows a significant improvement. Loss is smoothed with the wandb linear smoothing function.*

## S6: Results for only water-containing mixtures

During the n-fold cross-validation, we did not think that extrapolation towards water would be a likely use case and thus excluded water from $val_{ext}$. In the following, the results are shown for the fine-tuning

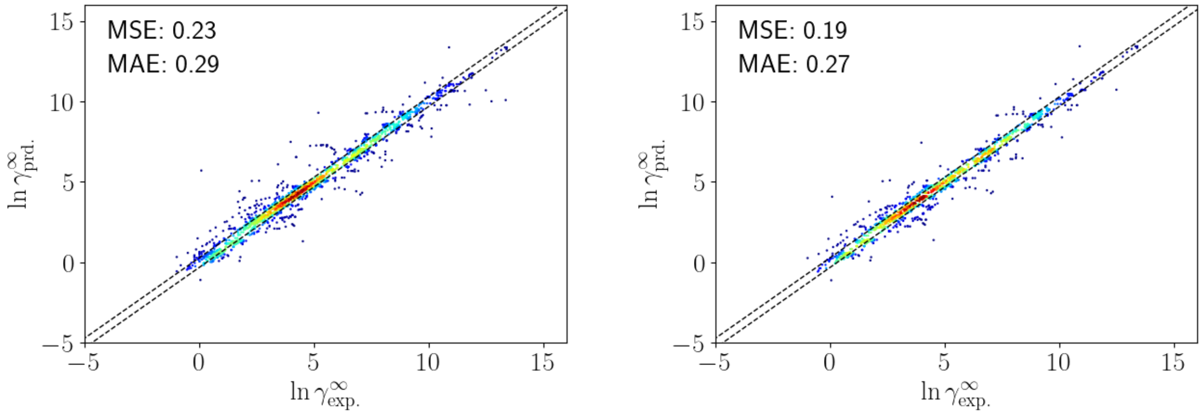


*Figure S3: Scatter plot of the n-fold cross validation on the Brouwer dataset for $Val_{edge}$ (left)and $Val_{int}$ (right) considering only mixtures that use water as solvent.*

in the sets $val_{int}$ (**Error! Reference source not found.** left) and $val_{edge}$ (**Error! Reference source not found.** right) for mixtures containing water as known solvent with an unknown solute. The model's performance is slightly worse than the overall assessment that contains all available mixtures. ($MSE_{int}$ 0.10 vs. 0.19 and $MSE_{edge}$ 0.14 vs. 0.23.) This result is likely due to the special characteristic of water, which makes predictions of property data difficult. Furthermore, as water is a molecule with a single character SMILES representation, the model cannot use knowledge about molecular structures in its prediction.

## S7: Comparison COMSO-SAC

In addition to COSMO-RS and UNIFAC, the results of our SPT model are compared to COSMO-SAC. For COSMO-SAC, we use the implementation of COSMO-SAC 2002 and COSMO-SAC dsp by Bell et al.[1] and the sigma profiles provided within this implementation by Fingerhut et al.[2] In both implementations, COMSO-SAC performed worse than any other predictive method with an $|\Delta \ln \gamma^{\infty}| < 0.3$ for 38% of mixtures for $\text{COSMO-SAC}_{2002}$, and 50% for $\text{COSMO-SAC}_{dsp}$

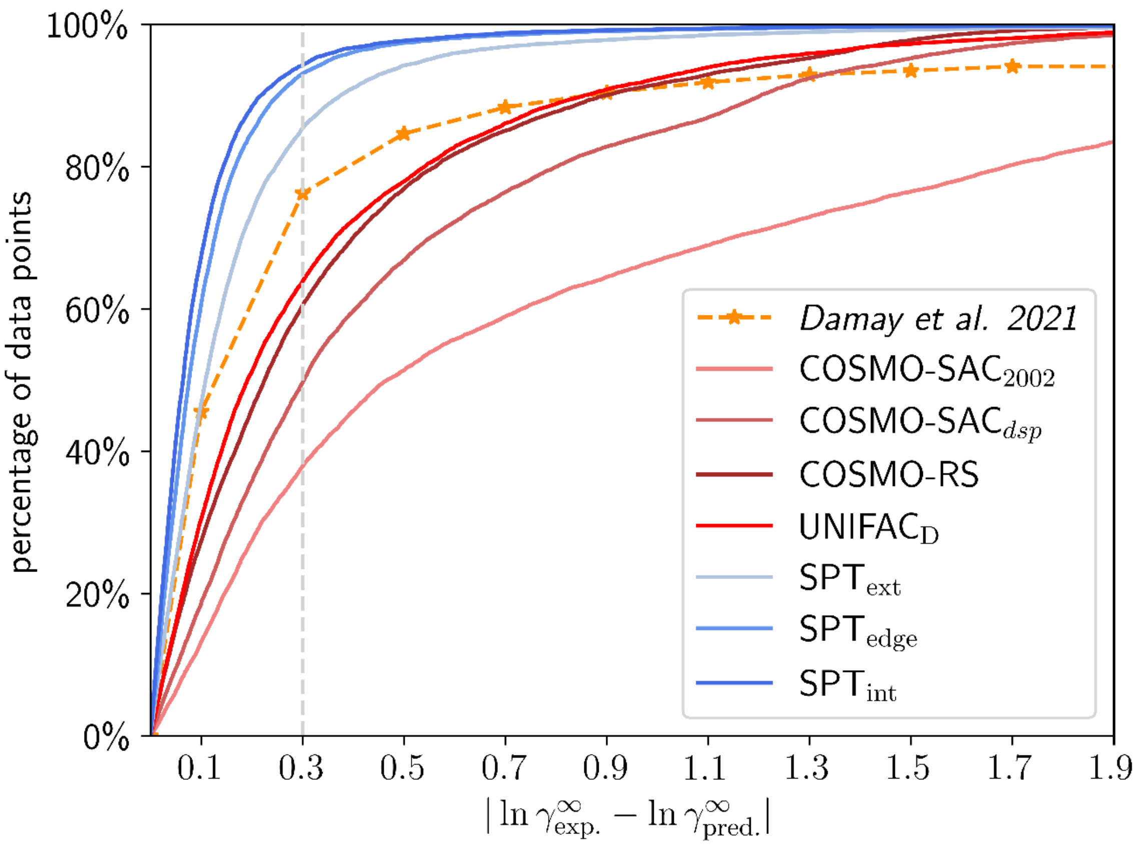


*Figure 4: Cumulative distribution of the prediction error $|\Delta \ln \gamma^{\infty}|$ over number of samples for COSMO-SAC, COSMO-RS, UNIFAC, $Val_{ext}$, $Val_{edge}$ and $Val_{int}$ using a common dataset. For $Val_{edge}$ and $Val_{int}$ the mean of the n-fold cross validation is used. Data for Damay et al. is approximated from their publication.*

## S8: Training of Sanchez Medina et al. model

Sanchez Medina et al.[3] released a machine learning model to predict limiting activity coefficients with all code and data available on their GitHub page: https://github.com/edgarsmdn/GNN_IAC.

To compare the performance of SPT to the model by Sanchez Medina et al., we reproduced their work but applied our method for splitting the data into 200 training and validation sets. Since this definition of training and validation sets is not 100% compatible with the training procedure by Sanchez Medina

et al., we had to make minor changes to their code. In the following text, we first describe the changes made to the code, followed by the training results.

The training procedure of Sanchez Medina et al. uses a test set to set the learning rate of the ML model. The learning rate is reduced once the loss of the training set does not decrease for more than three epochs. Furthermore, the model with the lowest test loss over the 200 epoch is considered the final model in the training code of Sanchez Medina et al. Since we do not have a training set for which we track the loss during training, both methods are not available to us.

To set the learning rate, we instead used the $Val_{ext}$ loss. To select the best model, we trained for 200 epochs on each training/validation set and then determined the lowest loss for each Validation set and selected this epoch as the final epoch for all models.

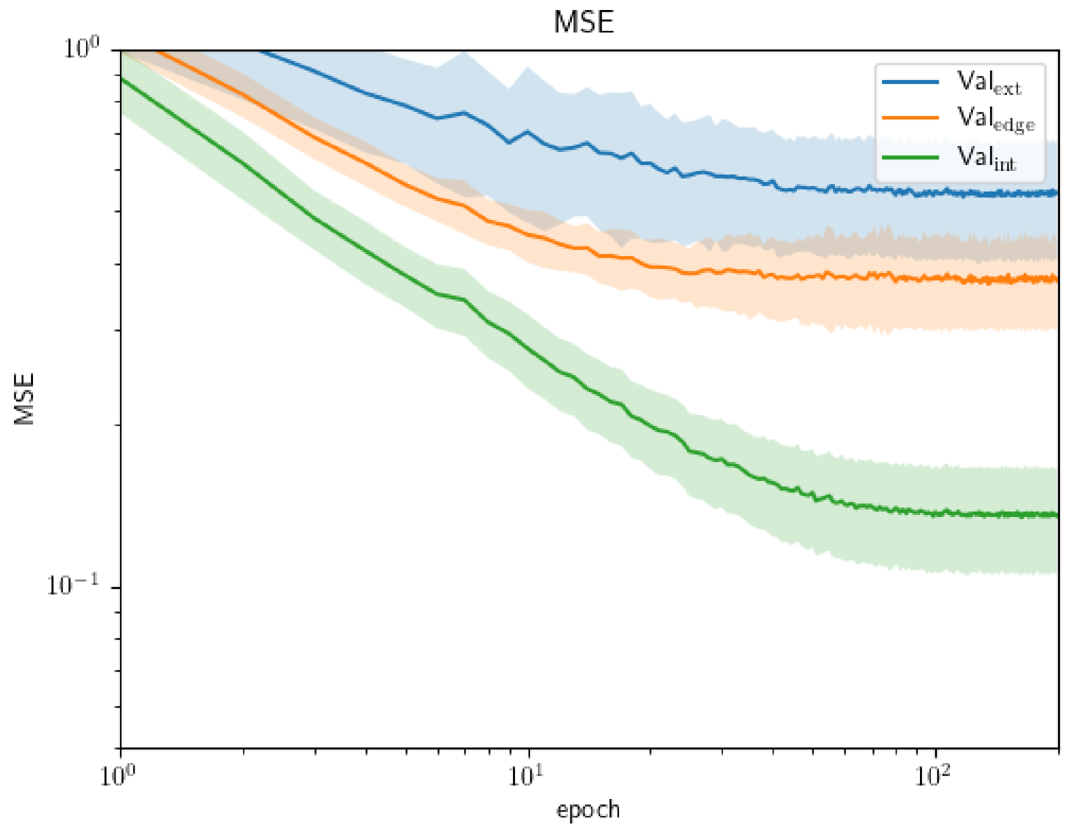


*Figure S5: Progression of loss for training the Medina model.*

Figure S1 shows the progression of $Val_{iext,}$ $Val_{edge}$, and $Val_{int}$ over 200 epochs.

## S9: Performance on all calculatable datapoints

*Table 4: Mean average error (MAE), mean square error (MSE), and the percentage of data with* $|\Delta ln\, \gamma^{\infty}| < 0.3$ *of the assessed models COSMO-RS, UNIFAC, Damay et al., Sanches Medina et al., and our model on the Brouwer and Medina datasets considering all points that can be calculated by each model. Results are thus not 100% comparable since each modle evelautes a different dataset. The model of Damay et al. does not include MAE and MSE as they are not disclosed in the original publication, and the model is not available for reproduction.*

| **Dataset** | Brouwer | | | Medina | | |
|---|---|---|---|---|---|---|
| **Error** | MAE | MSE | $\|\Delta \ln\gamma\| < 0.3$ | MEA | MSE | $\|\Delta \ln\gamma\| < 0.3$ |
| COSMO-RS | 0.38 | 0.36 | 56.6% | 0.31 | 0.24 | 64.5% |
| UNIFAC | 0.59 | 0.85 | 52.8% | 0.28 | 0.33 | 74.5% |
| *Damay et al.* | - | - | *(76.6%)* | | | |
| $\text{Medina}_{ext}$ | | | | 0.48 | 0.53 | 50.1% |
| $\text{Medina}_{edge}$ | | | | 0.29 | 0.21 | 67.2% |
| $\text{Medina}_{int}$ | | | | 0.19 | 0.10 | 83.1% |
| $\text{SPT}_{ext}$ | **0.20** | **0.13** | **80.8%** | **0.25** | **0.18** | **74.6%** |
| $\text{SPT}_{edge}$ | **0.16** | **0.08** | **88.2%** | **0.17** | **0.08** | **85.7%** |
| $\text{SPT}_{int}$ | **0.13** | **0.06** | **91.3%** | **0.13** | **0.05** | **92.5%** |

## References


1 I. H. Bell, E. Mickoleit, C.-M. Hsieh, S.-T. Lin, J. Vrabec, C. Breitkopf and A. Jäger, *Journal of chemical theory and computation*, 2020, **16**, 2635–2646.

2 R. Fingerhut, W.-L. Chen, A. Schedemann, W. Cordes, J. Rarey, C.-M. Hsieh, J. Vrabec and S.-T. Lin, *Ind. Eng. Chem. Res.*, 2017, **56**, 9868–9884.

3 E. I. Sanchez Medina, S. Linke, M. Stoll and K. Sundmacher, *Digital Discovery*, 2022.
